# Supplementary material for: H3DNet: 3D Object Detection Using Hybrid Geometric Primitives
Source: arXiv:2006.05682 source file (2020-07-23)
Supplement: Supplementary file 2 [file 10_supp_proof.tex]

\section{Proof of Proposition 1}
\label{Section::Supp:proof}
We show the proof of Proposition 1 here.

With chain rule and equation (3) in the main paper, we can directly get:
\begin{equation}
    \frac{\partial l_m}{\partial \Theta}= 2(\bs{x}_{\Theta}^{\star}-\bs{x}^{\gt})^T\cdot \frac{\partial \bs{x}_{\Theta}^{\star}}{\partial \Theta} .
\end{equation}

Since $\bs{x}^{\star}$ is the local minimum of $f_{\Theta}(\bs{x})$, we have:
\begin{equation}
    \frac{\partial f_{\Theta}(\bs{x}^{\star})}{\partial \bs{x}} = 0 .
\end{equation}

Compute the derivatives of both sides w.r.t. $\Theta$, i.e. 
\begin{equation}
    \frac{\partial^2 f_{\Theta}(\bs{x}^{\star})}{\partial^2 \bs{x}} \cdot \frac{\partial \bs{x}^{\star}}{\partial \Theta} + \frac{\partial^2 f_{\Theta}(\bs{x}^{\star})}{\partial \bs{x}\partial \Theta} = 0 ,
\end{equation}
which leads to the equation (4) in the main paper.
% \begin{proposition}
% The derivatives of $l_m$ with respect to $\Theta$ is given by
% \begin{equation}
% \frac{\partial l_m}{\partial \Theta}:= 2(\bs{x}_{\Theta}^{\star}-\bs{x}^{\gt})^T\cdot \frac{\partial \bs{x}_{\Theta}^{\star}}{\partial \Theta},\quad \frac{\partial \bs{x}_{\Theta}^{\star}}{\partial \Theta}:= -\Big(\frac{\partial^2 f_{\Theta}(\bs{x}^{\star})}{\partial^2 \bs{x}}\Big)^{-1}\cdot \frac{\partial^2 f_{\Theta}(\bs{x}^{\star})}{\partial \bs{x}\partial \Theta}.
% \label{Eq:Derivatives}
% \end{equation}
% \label{Prop:IFM}
% \vspace{-0.25in}
% \end{proposition}
